# Supplementary material for: Pay Attention to What and Where? Interpretable Feature Extractor in Vision-based Deep Reinforcement Learning
Source: arXiv:2504.10071 source file (2025-04-14)
Supplement: Supplementary file 1 [file 07-appendix.tex]

\appendix
\section{Appendix / supplemental material}
\subsection{Network Architectures}
\label{append:network_arch}
